# Supplementary material for: Block Decomposable Methods for Large-Scale Optimization Problems
Source: arXiv:2601.09010 source file (2026-01-13)
Supplement: Supplementary file 2 [file appendix1.tex]

%%%%%%%%%%%%%%%%%%%%%%%%%%%%%%%%%%%%%%%%%%%%%%%%%%%
%
%  New template code for TAMU Theses and Dissertations starting Spring 2021.
%
%
%  Author: Thesis Office 
%	 
%  Last updated 1/13/2021
%
%%%%%%%%%%%%%%%%%%%%%%%%%%%%%%%%%%%%%%%%%%%%%%%%%%%

%%%%%%%%%%%%%%%%%%%%%%%%%%%%%%%%%%%%%%%%%%%%%%%%%%%%%%%%%%%%%%%%%%%%%%
%%                           APPENDIX A 
%%%%%%%%%%%%%%%%%%%%%%%%%%%%%%%%%%%%%%%%%%%%%%%%%%%%%%%%%%%%%%%%%%%%%

\phantomsection

\chapter{\uppercase{First Appendix}}

Text for the Appendix follows.

\begin{figure}[h]
\centering
\includegraphics[scale=.50]{figures/Penguins.jpg}
\caption{TAMU figure}
\label{fig:tamu-fig5}
\end{figure}
